# Supplementary material for: Federated Learning Enables Big Data for Rare Cancer Boundary Detection
Source: arXiv:2204.10836 source file (2022-04-25)
Supplement: Supplementary file 1 [file 5_supplementary.tex]

            % 13 EXTENDED DATA FIGURE/TABLE LEGENDS (% ACCORDING TO NATURE)
\begin{figure}
    \centering
    \begin{subfigure}[t]{0.03\textwidth}
    \textbf{a}
    \end{subfigure}
    \begin{subfigure}[t]{0.7\textwidth}
        \includegraphics[width=\textwidth, valign=t]{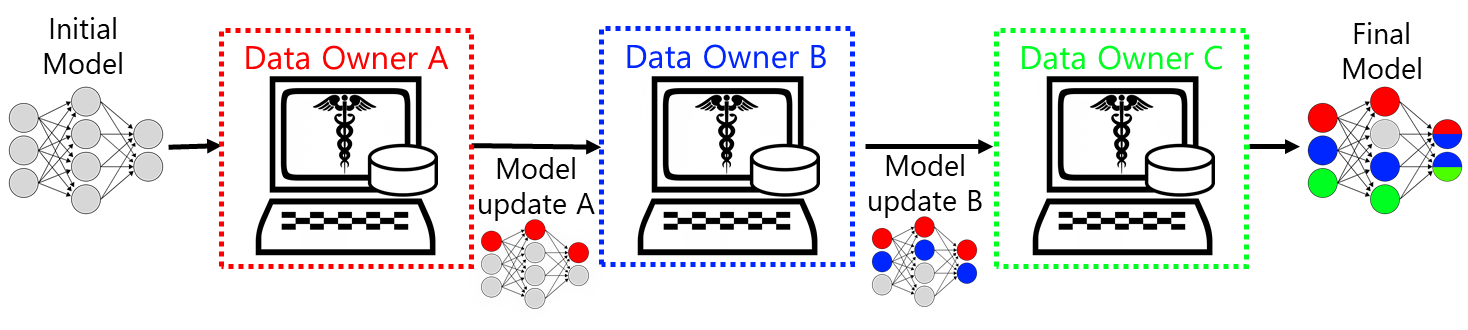}
    \end{subfigure}
    \\
    \begin{subfigure}[t]{0.03\textwidth}
    \textbf{b}
    \end{subfigure}
    \begin{subfigure}[t]{0.7\textwidth}
        \includegraphics[width=\textwidth, valign=t]{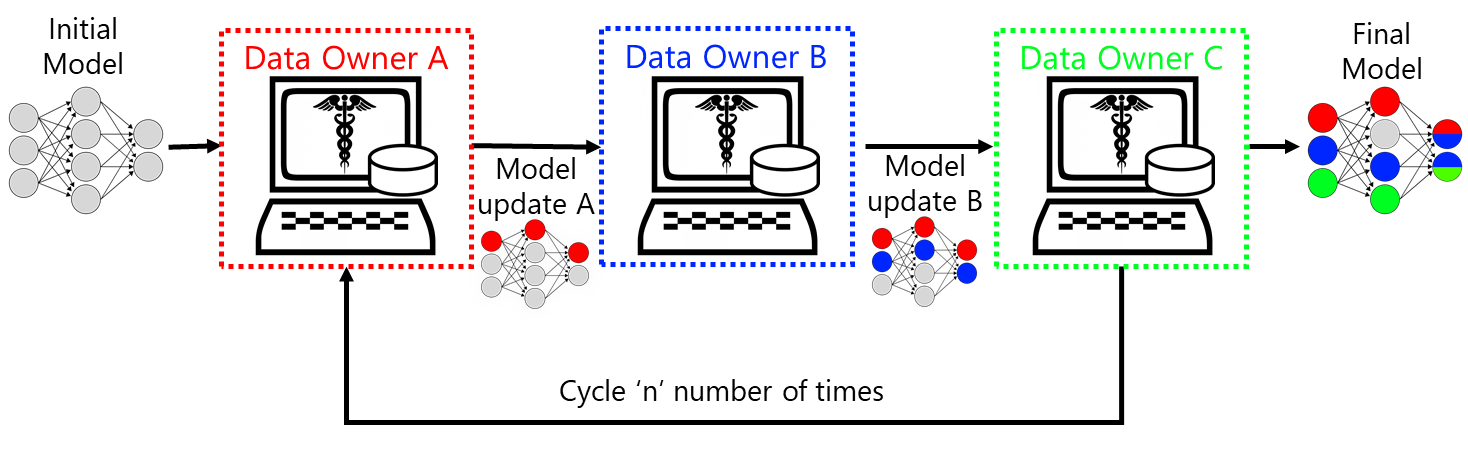}
    \end{subfigure}
    \\
    \begin{subfigure}[t]{0.03\textwidth}
    \textbf{c}
    \end{subfigure}
    \begin{subfigure}[t]{0.45\textwidth}
        \includegraphics[width=\textwidth, valign=t]{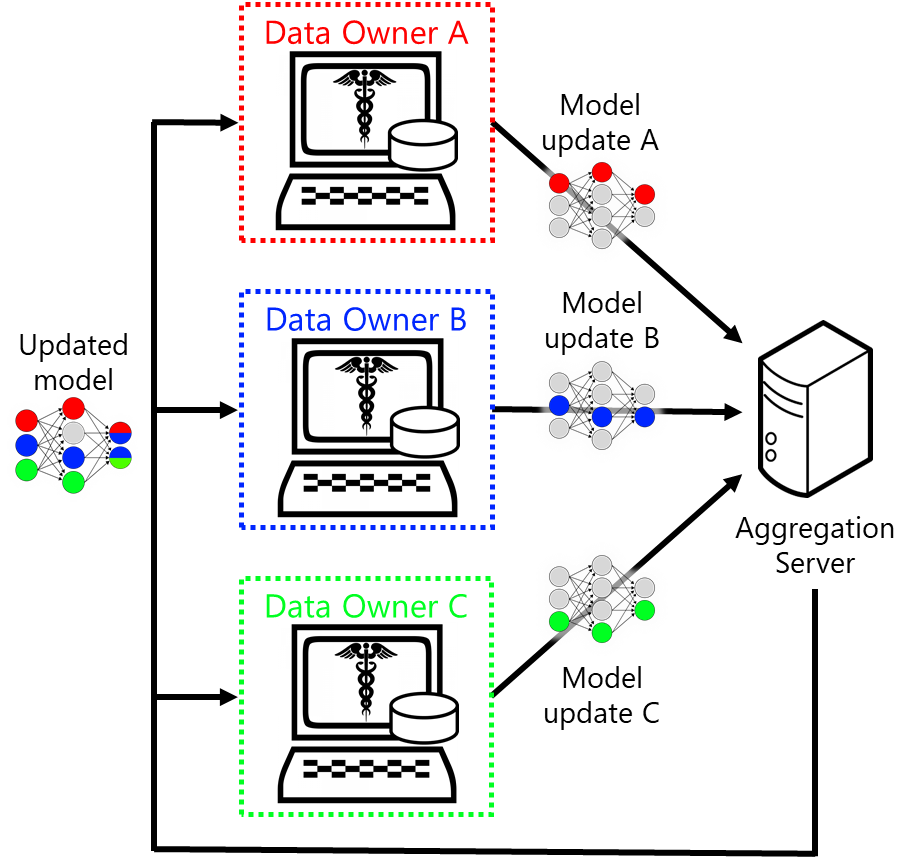}
    \end{subfigure}
    \hfill
    \begin{subfigure}[t]{0.03\textwidth}
    \textbf{d}
    \end{subfigure}
    \begin{subfigure}[t]{0.45\textwidth}
        \includegraphics[width=\textwidth, valign=t]{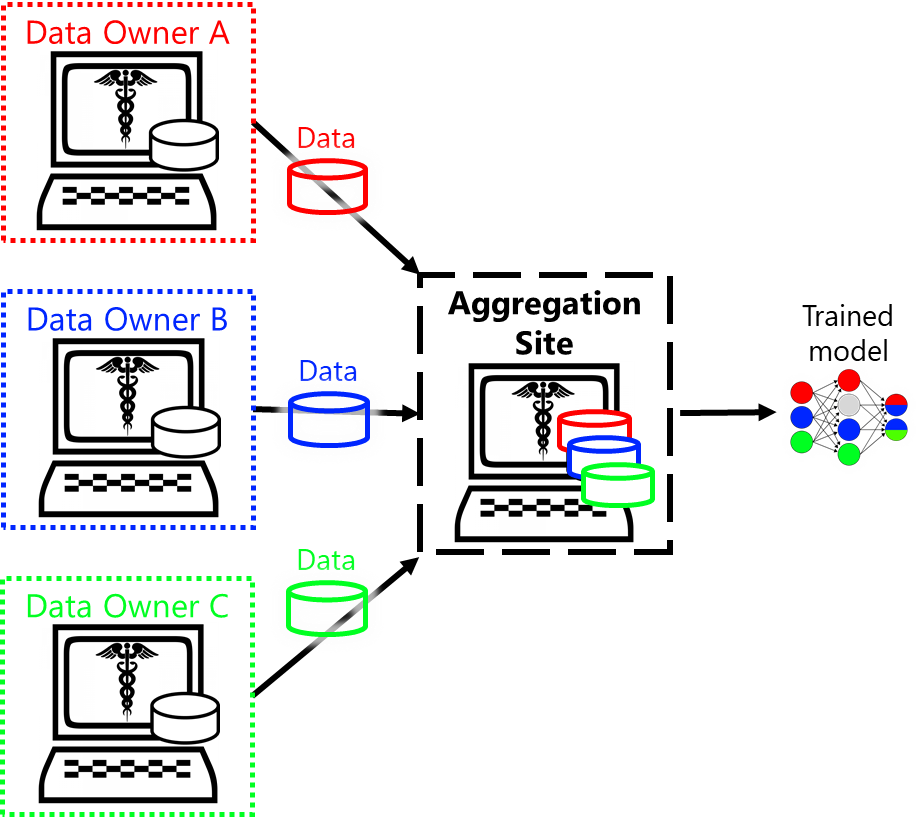}
    \end{subfigure}
    \caption{Illustration of the different approaches to train DL models during multi-site collaborations. \textbf{a}, Institutional incremental learning (IIL). \textbf{b}, Cyclic Institutional incremental learning. \textbf{c}, Federated learning by independent aggregation. \textbf{d}, Centralized learning by aggregating data.}
    \label{fig:fl_approaches}
    \label{fig:fl_approaches:afl}
\end{figure}

%% SP on 2022/02/23: for some reason, if this is defined once, it doesn't show up
\begin{figure}
  \centering
  \includegraphics[width=1.0\textwidth, valign=t]{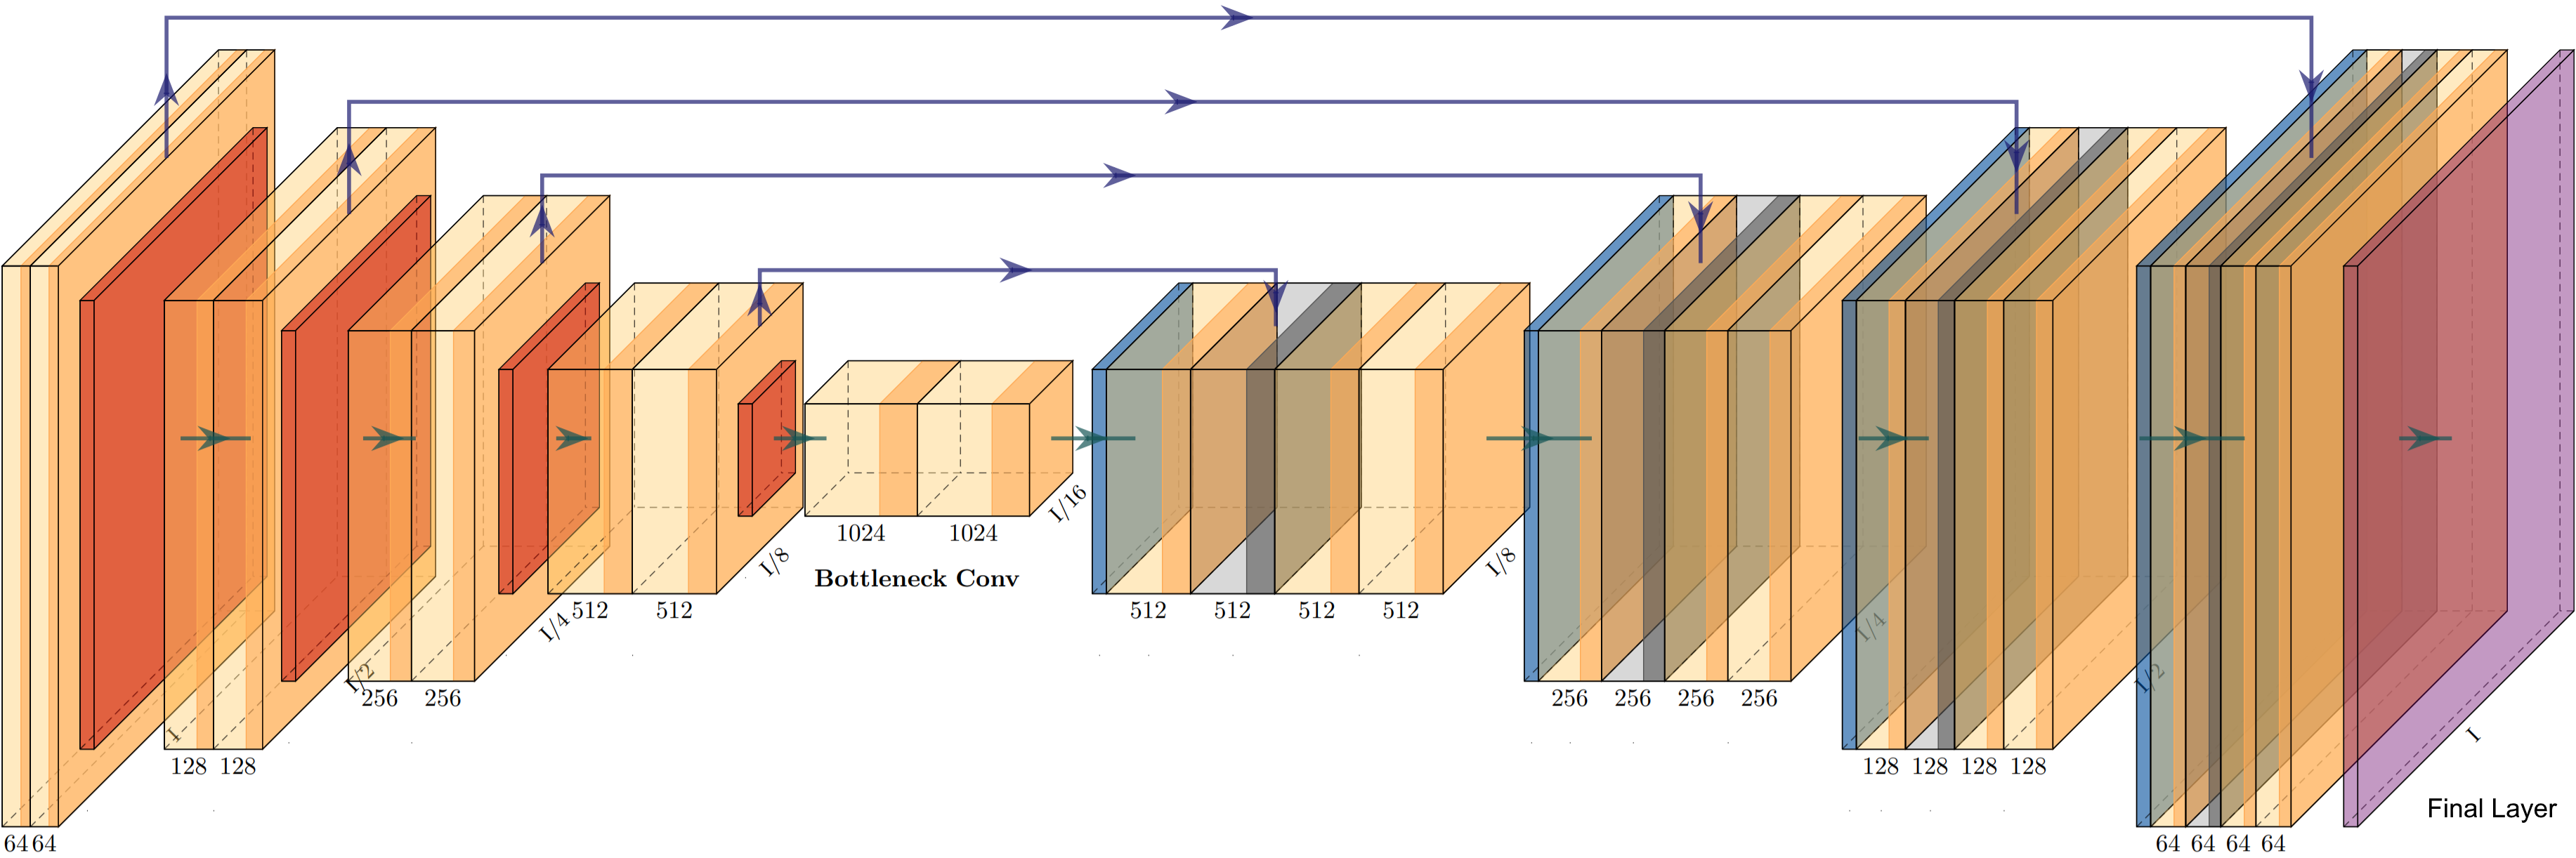}
  \caption{Illustration of the U-Net architecture with residual connections, plotted using PlotNeuralNet \url{https://github.com/HarisIqbal88/PlotNeuralNet}. One spatial dimension is left out for clarity.}
  \label{fig:unet}
\end{figure}

\begin{figure}[t]
    \centering
    \includegraphics[width=0.5\textwidth, valign=t]{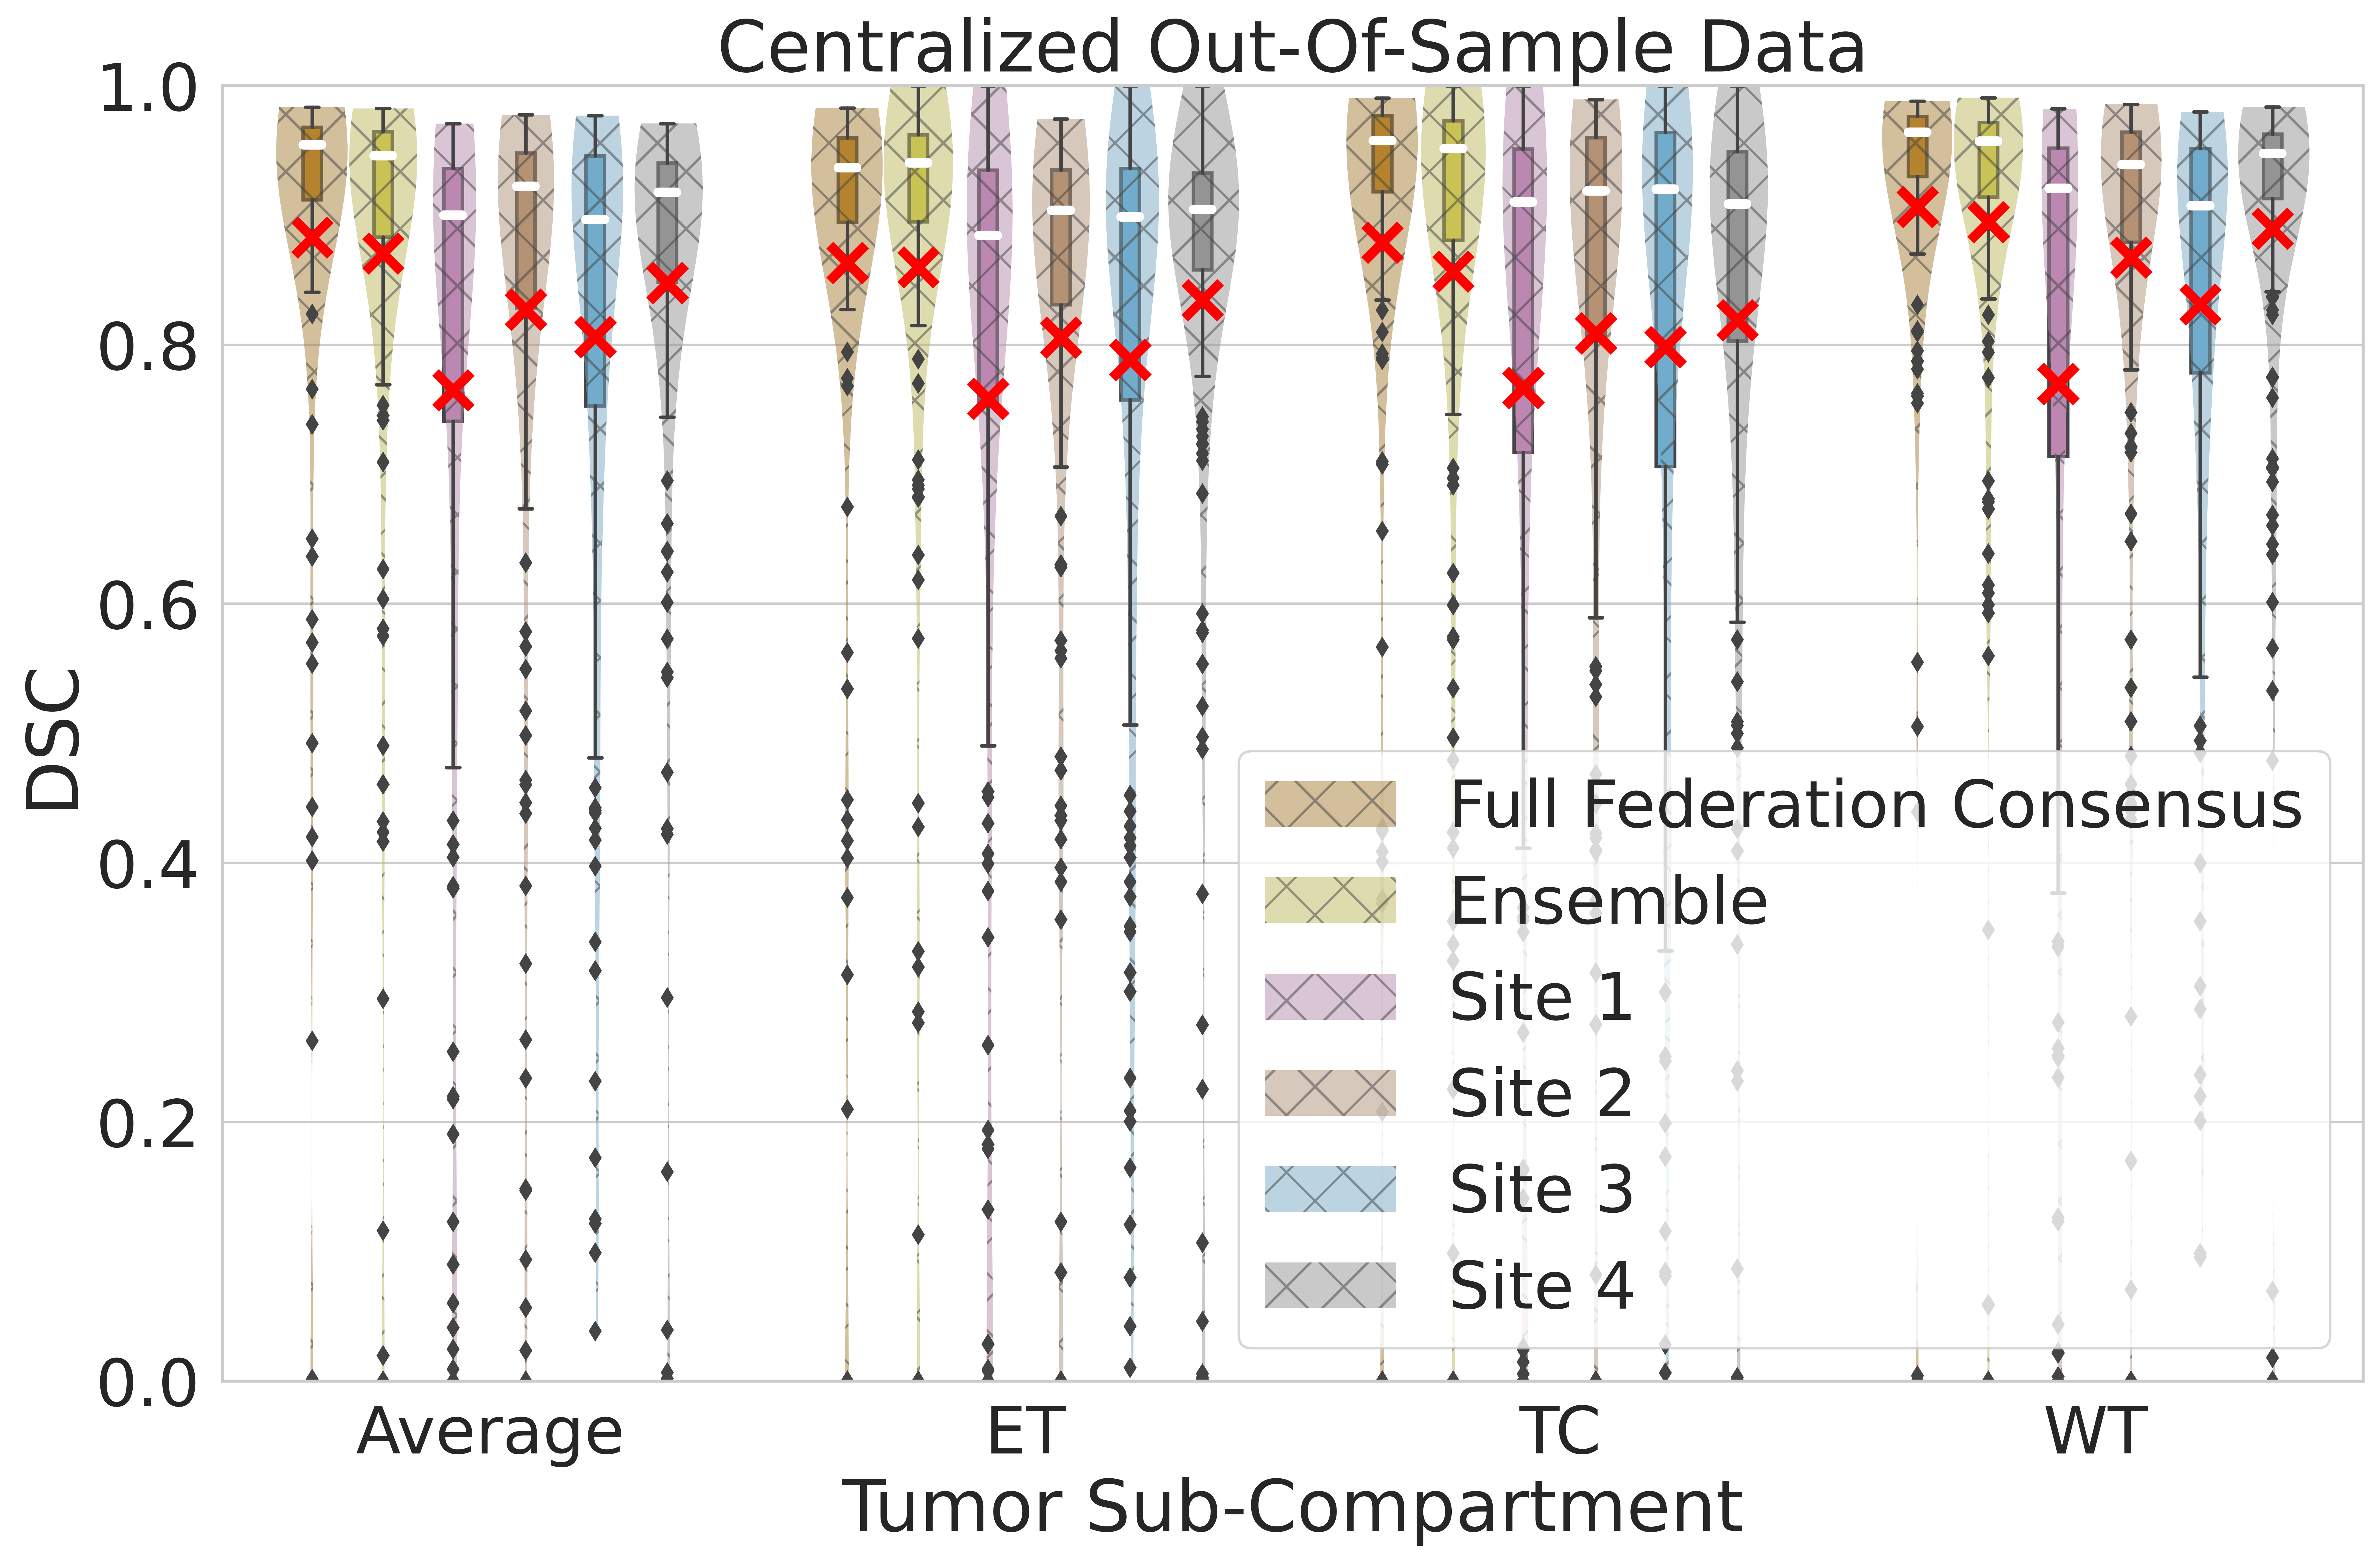}
    \caption{Comparative performance evaluation of the final consensus model, per tumor sub-compartment and averaged across cases. Comparison with the public initial model with each single site model (for collaborators holding $>200$ samples), as well as with their ensemble. Significance of results (Wilcoxon signed-rank test): Site 1: $p_{Average}=2\times 10^{-7}$, $p_{ET}=4\times 10^{-8}$, $p_{TC}=6\times 10^{-8}$, $p_{WT}=2\times 10^{-9}$; Site 2: $p_{Average}=5\times 10^{-6}$, $p_{ET}=1\times 10^{-5}$, $p_{TC}=1\times 10^{-4}$, $p_{WT}=1\times 10^{-4}$, Site 3: $p_{Average}=3\times 10^{-7}$, $p_{ET}=2\times 10^{-6}$, $p_{TC}=1\times 10^{-6}$, $p_{WT}=6\times 10^{-9}$, Site 4: $p_{Average}=4\times 10^{-6}$, $p_{ET}=5\times 10^{-5}$, $p_{TC}=8\times 10^{-7}$, $p_{WT}=8\times 10^{-3}$.}
    \label{fig:single_and_consensus_models_against_holdout_singles}
\end{figure}

\begin{table}
\centering
\caption{Average $DSC$ over cases for various \textit{singlet} and \textit{triplet} models against the centralized out-of-sample data}
\label{tab:results_singlet-triplet}
\begin{tabular}{|cc|cccc|}
\hline
\multicolumn{2}{|c|}{\textbf{Model}} &
  \multicolumn{4}{c|}{$DSC$} \\ \hline
\multicolumn{1}{|c|}{\textbf{Type}} &
  \textbf{Index} &
  \multicolumn{1}{c|}{\textbf{Average}} &
  \multicolumn{1}{c|}{\textbf{ET}} &
  \multicolumn{1}{c|}{\textbf{TC}} &
  \textbf{WT} \\ \hline
\multicolumn{1}{|c|}{\multirow{5}{*}{\textbf{\textit{singlet}}}} &
  0 &
  \multicolumn{1}{c|}{0.743996} &
  \multicolumn{1}{c|}{0.683714} &
  \multicolumn{1}{c|}{0.713348} &
  0.834925 \\ \cline{2-6} 
\multicolumn{1}{|c|}{} &
  1 &
  \multicolumn{1}{c|}{0.745362} &
  \multicolumn{1}{c|}{0.690743} &
  \multicolumn{1}{c|}{0.714308} &
  0.831035 \\ \cline{2-6} 
\multicolumn{1}{|c|}{} &
  2 &
  \multicolumn{1}{c|}{0.742246} &
  \multicolumn{1}{c|}{0.6806} &
  \multicolumn{1}{c|}{0.711266} &
  0.834871 \\ \cline{2-6} 
\multicolumn{1}{|c|}{} &
  3 &
  \multicolumn{1}{c|}{0.745255} &
  \multicolumn{1}{c|}{0.697808} &
  \multicolumn{1}{c|}{0.710747} &
  0.82721 \\ \cline{2-6} 
\multicolumn{1}{|c|}{} &
  4 &
  \multicolumn{1}{c|}{0.74213} &
  \multicolumn{1}{c|}{0.687588} &
  \multicolumn{1}{c|}{0.711013} &
  0.827789 \\ \hline
\multicolumn{1}{|c|}{\multirow{5}{*}{\textbf{\textit{triplet}}}} &
  0 &
  \multicolumn{1}{c|}{0.749014} &
  \multicolumn{1}{c|}{0.697808} &
  \multicolumn{1}{c|}{0.714308} &
  0.834925 \\ \cline{2-6} 
\multicolumn{1}{|c|}{} &
  1 &
  \multicolumn{1}{c|}{0.750356} &
  \multicolumn{1}{c|}{0.697808} &
  \multicolumn{1}{c|}{0.718336} &
  0.834925 \\ \cline{2-6} 
\multicolumn{1}{|c|}{} &
  2 &
  \multicolumn{1}{c|}{0.748694} &
  \multicolumn{1}{c|}{0.697808} &
  \multicolumn{1}{c|}{0.713348} &
  0.834925 \\ \cline{2-6} 
\multicolumn{1}{|c|}{} &
  3 &
  \multicolumn{1}{c|}{0.748996} &
  \multicolumn{1}{c|}{0.697808} &
  \multicolumn{1}{c|}{0.714308} &
  0.834871 \\ \cline{2-6} 
\multicolumn{1}{|c|}{} &
  4 &
  \multicolumn{1}{c|}{0.746683} &
  \multicolumn{1}{c|}{0.697808} &
  \multicolumn{1}{c|}{0.714308} &
  0.827934 \\ \hline
\end{tabular}
\end{table}

\begin{table}
\centering
\caption{P values providing significance of the difference in mean $DSC$ scores across cases between each \textit{singlet} and \textit{triplet} model pairing on the centralized out-of-sample data. Significance is calculated using Wilcoxon signed-ranked test where sample pairs are correspondingly the \textit{singlet} and \textit{triplet} model score for a single case. Entries with `NA' correspond to scoring where the \textit{singlet} model was the member of the \textit{triplet} responsible for producing the particular tumor sub-compartment output, so that the scores between the \textit{singlet} and the \textit{triplet} model for that tumor sub-compartment were identical.}
\label{tab:results_singlet-triplet_full}
\begin{tabular}{|cc|ccccc|}
\hline
\multicolumn{2}{|c|}{\textbf{}} &
  \multicolumn{5}{c|}{\textbf{\textit{singlet} Index}} \\ \hline
\multicolumn{1}{|c|}{\textbf{\begin{tabular}[c]{@{}c@{}}\textbf{\textit{triplet}}\\ Index\end{tabular}}} &
  \textbf{metric} &
  \multicolumn{1}{c|}{\textbf{0}} &
  \multicolumn{1}{c|}{\textbf{1}} &
  \multicolumn{1}{c|}{\textbf{2}} &
  \multicolumn{1}{c|}{\textbf{3}} &
  4 \\ \hline
\multicolumn{1}{|c|}{\multirow{4}{*}{0}} &
  Average &
  \multicolumn{1}{c|}{$5.9\times10^{-6}$} &
  \multicolumn{1}{c|}{0.31} &
  \multicolumn{1}{c|}{$8.3\times10^{-12}$} &
  \multicolumn{1}{c|}{0.21} &
  $1.8\times10^{-6}$ \\ \cline{2-7} 
\multicolumn{1}{|c|}{} &
  ET &
  \multicolumn{1}{c|}{$3.2\times10^{-19}$} &
  \multicolumn{1}{c|}{$5.1\times10^{-6}$} &
  \multicolumn{1}{c|}{$3.7\times10^{-17}$} &
  \multicolumn{1}{c|}{NA} &
  $2.3\times10^{-22}$ \\ \cline{2-7} 
\multicolumn{1}{|c|}{} &
  TC &
  \multicolumn{1}{c|}{0.35} &
  \multicolumn{1}{c|}{NA} &
  \multicolumn{1}{c|}{$2.3\times10^{-6}$} &
  \multicolumn{1}{c|}{0.37} &
  0.76 \\ \cline{2-7} 
\multicolumn{1}{|c|}{} &
  WT &
  \multicolumn{1}{c|}{NA} &
  \multicolumn{1}{c|}{0.34} &
  \multicolumn{1}{c|}{0.026} &
  \multicolumn{1}{c|}{0.61} &
  0.00037 \\ \hline
\multicolumn{1}{|c|}{\multirow{4}{*}{1}} &
  Average &
  \multicolumn{1}{c|}{$5.5\times10^{-11}$} &
  \multicolumn{1}{c|}{0.0047} &
  \multicolumn{1}{c|}{$1.6\times10^{-16}$} &
  \multicolumn{1}{c|}{0.0017} &
  $1.1\times10^{-13}$ \\ \cline{2-7} 
\multicolumn{1}{|c|}{} &
  ET &
  \multicolumn{1}{c|}{$3.2\times10^{-19}$} &
  \multicolumn{1}{c|}{$5.1\times10^{-6}$} &
  \multicolumn{1}{c|}{$3.7\times10^{-17}$} &
  \multicolumn{1}{c|}{NA} &
  $2.3\times10^{-22}$ \\ \cline{2-7} 
\multicolumn{1}{|c|}{} &
  TC &
  \multicolumn{1}{c|}{0.012} &
  \multicolumn{1}{c|}{0.013} &
  \multicolumn{1}{c|}{$2.4\times10^{-9}$} &
  \multicolumn{1}{c|}{0.027} &
  0.016 \\ \cline{2-7} 
\multicolumn{1}{|c|}{} &
  WT &
  \multicolumn{1}{c|}{NA} &
  \multicolumn{1}{c|}{0.34} &
  \multicolumn{1}{c|}{0.026} &
  \multicolumn{1}{c|}{0.61} &
  0.00037 \\ \hline
\multicolumn{1}{|c|}{\multirow{4}{*}{2}} &
  Average &
  \multicolumn{1}{c|}{$4.3\times10^{-19}$} &
  \multicolumn{1}{c|}{0.97} &
  \multicolumn{1}{l|}{$7.0\times10^{-13}$} &
  \multicolumn{1}{c|}{0.21} &
  $6.4\times10^{-6}$ \\ \cline{2-7} 
\multicolumn{1}{|c|}{} &
  ET &
  \multicolumn{1}{c|}{$3.2\times10^{-19}$} &
  \multicolumn{1}{c|}{$5.1\times10^{-6}$} &
  \multicolumn{1}{c|}{$3.7\times10^{-17}$} &
  \multicolumn{1}{c|}{NA} &
  $2.3\times10^{-22}$ \\ \cline{2-7} 
\multicolumn{1}{|c|}{} &
  TC &
  \multicolumn{1}{c|}{NA} &
  \multicolumn{1}{c|}{0.35} &
  \multicolumn{1}{l|}{$2.6\times10^{-8}$} &
  \multicolumn{1}{c|}{0.83} &
  0.29 \\ \cline{2-7} 
\multicolumn{1}{|c|}{} &
  WT &
  \multicolumn{1}{c|}{NA} &
  \multicolumn{1}{c|}{0.34} &
  \multicolumn{1}{c|}{0.026} &
  \multicolumn{1}{c|}{0.61} &
  0.00037 \\ \hline
\multicolumn{1}{|c|}{\multirow{4}{*}{3}} &
  Average &
  \multicolumn{1}{c|}{0.0021} &
  \multicolumn{1}{c|}{0.57} &
  \multicolumn{1}{l|}{$1.9\times10^{-11}$} &
  \multicolumn{1}{c|}{0.87} &
  $4.6\times10^{-5}$ \\ \cline{2-7} 
\multicolumn{1}{|c|}{} &
  ET &
  \multicolumn{1}{c|}{$3.2\times10^{-19}$} &
  \multicolumn{1}{c|}{$5.1\times10^{-6}$} &
  \multicolumn{1}{c|}{$3.7\times10^{-17}$} &
  \multicolumn{1}{c|}{NA} &
  $2.3\times10^{-22}$ \\ \cline{2-7} 
\multicolumn{1}{|c|}{} &
  TC &
  \multicolumn{1}{c|}{0.35} &
  \multicolumn{1}{c|}{NA} &
  \multicolumn{1}{c|}{$2.3\times10^{-6}$} &
  \multicolumn{1}{c|}{0.37} &
  0.76 \\ \cline{2-7} 
\multicolumn{1}{|c|}{} &
  WT &
  \multicolumn{1}{c|}{0.026} &
  \multicolumn{1}{c|}{0.00071} &
  \multicolumn{1}{c|}{NA} &
  \multicolumn{1}{c|}{0.24} &
  0.88 \\ \hline
\multicolumn{1}{|c|}{\multirow{4}{*}{4}} &
  Average &
  \multicolumn{1}{c|}{0.53} &
  \multicolumn{1}{c|}{$6.5\times10^{-8}$} &
  \multicolumn{1}{c|}{0.16} &
  \multicolumn{1}{c|}{0.0094} &
  0.77 \\ \cline{2-7} 
\multicolumn{1}{|c|}{} &
  ET &
  \multicolumn{1}{c|}{$3.2\times10^{-19}$} &
  \multicolumn{1}{c|}{$5.1\times10^{-6}$} &
  \multicolumn{1}{c|}{$3.7\times10^{-17}$} &
  \multicolumn{1}{c|}{NA} &
  $2.3\times10^{-22}$ \\ \cline{2-7} 
\multicolumn{1}{|c|}{} &
  TC &
  \multicolumn{1}{c|}{0.35} &
  \multicolumn{1}{c|}{NA} &
  \multicolumn{1}{c|}{$2.3\times10^{-6}$} &
  \multicolumn{1}{c|}{0.37} &
  0.76 \\ \cline{2-7} 
\multicolumn{1}{|c|}{} &
  WT &
  \multicolumn{1}{c|}{$4.0\times10^{-26}$} &
  \multicolumn{1}{c|}{$7.7\times10^{-21}$} &
  \multicolumn{1}{c|}{$3.7\times10^{-24}$} &
  \multicolumn{1}{c|}{$4.9\times10^{-10}$} &
  $1.3\times10^{-12}$ \\ \hline
\end{tabular}
\end{table}

\begin{table}
\caption{Demographic information of all cases used in this study.}
\label{tab:demographics}
\begin{adjustbox}{width=\textwidth,totalheight=\textheight,keepaspectratio}
\centering

\begin{tabular}{|
>{\columncolor[HTML]{FFFFFF}}c |
>{\columncolor[HTML]{FFFFFF}}c |
>{\columncolor[HTML]{FFFFFF}}c 
>{\columncolor[HTML]{FFFFFF}}c 
>{\columncolor[HTML]{FFFFFF}}c |
>{\columncolor[HTML]{FFFFFF}}c 
>{\columncolor[HTML]{FFFFFF}}c 
>{\columncolor[HTML]{FFFFFF}}c 
>{\columncolor[HTML]{FFFFFF}}c |
>{\columncolor[HTML]{FFFFFF}}c 
>{\columncolor[HTML]{FFFFFF}}c 
>{\columncolor[HTML]{FFFFFF}}c 
>{\columncolor[HTML]{FFFFFF}}c |
>{\columncolor[HTML]{FFFFFF}}c 
>{\columncolor[HTML]{FFFFFF}}c 
>{\columncolor[HTML]{FFFFFF}}c |}
\hline
\cellcolor[HTML]{FFFFFF} &
  \cellcolor[HTML]{FFFFFF} &
  \multicolumn{3}{c|}{\cellcolor[HTML]{FFFFFF}\textbf{SEX}} &
  \multicolumn{4}{c|}{\cellcolor[HTML]{FFFFFF}\textbf{AGE: Male}} &
  \multicolumn{4}{c|}{\cellcolor[HTML]{FFFFFF}\textbf{AGE: Female}} &
  \multicolumn{3}{c|}{\cellcolor[HTML]{FFFFFF}\textbf{IDH status}} \\ \cline{3-16} 
\multirow{-2}{*}{\cellcolor[HTML]{FFFFFF}\textbf{Site ID}} &
  \multirow{-2}{*}{\cellcolor[HTML]{FFFFFF}\textbf{\begin{tabular}[c]{@{}c@{}}Total\\ Cases\end{tabular}}} &
  \multicolumn{1}{c|}{\cellcolor[HTML]{FFFFFF}\textbf{M}} &
  \multicolumn{1}{c|}{\cellcolor[HTML]{FFFFFF}\textbf{F}} &
  \textbf{NA} &
  \multicolumn{1}{c|}{\cellcolor[HTML]{FFFFFF}\textbf{Average}} &
  \multicolumn{1}{c|}{\cellcolor[HTML]{FFFFFF}\textbf{Std.Dev}} &
  \multicolumn{1}{c|}{\cellcolor[HTML]{FFFFFF}\textbf{Min}} &
  \textbf{Max} &
  \multicolumn{1}{c|}{\cellcolor[HTML]{FFFFFF}\textbf{Average}} &
  \multicolumn{1}{c|}{\cellcolor[HTML]{FFFFFF}\textbf{Std.Dev}} &
  \multicolumn{1}{c|}{\cellcolor[HTML]{FFFFFF}\textbf{Min}} &
  \textbf{Max} &
  \multicolumn{1}{c|}{\cellcolor[HTML]{FFFFFF}\textbf{mutant}} &
  \multicolumn{1}{c|}{\cellcolor[HTML]{FFFFFF}\textbf{wildtype}} &
  \textbf{NOS} \\ \hline
1 &
  827 &
  \multicolumn{1}{c|}{\cellcolor[HTML]{FFFFFF}495} &
  \multicolumn{1}{c|}{\cellcolor[HTML]{FFFFFF}332} &
  0 &
  \multicolumn{1}{c|}{\cellcolor[HTML]{FFFFFF}59.93} &
  \multicolumn{1}{c|}{\cellcolor[HTML]{FFFFFF}14.57} &
  \multicolumn{1}{c|}{\cellcolor[HTML]{FFFFFF}10} &
  89 &
  \multicolumn{1}{c|}{\cellcolor[HTML]{FFFFFF}61.22} &
  \multicolumn{1}{c|}{\cellcolor[HTML]{FFFFFF}13.55} &
  \multicolumn{1}{c|}{\cellcolor[HTML]{FFFFFF}20} &
  86 &
  \multicolumn{1}{c|}{\cellcolor[HTML]{FFFFFF}96} &
  \multicolumn{1}{c|}{\cellcolor[HTML]{FFFFFF}482} &
  249 \\ \hline
2 &
  611 &
  \multicolumn{1}{c|}{\cellcolor[HTML]{FFFFFF}367} &
  \multicolumn{1}{c|}{\cellcolor[HTML]{FFFFFF}244} &
  0 &
  \multicolumn{1}{c|}{\cellcolor[HTML]{FFFFFF}62.32} &
  \multicolumn{1}{c|}{\cellcolor[HTML]{FFFFFF}12.43} &
  \multicolumn{1}{c|}{\cellcolor[HTML]{FFFFFF}18.65} &
  87.59 &
  \multicolumn{1}{c|}{\cellcolor[HTML]{FFFFFF}64.03} &
  \multicolumn{1}{c|}{\cellcolor[HTML]{FFFFFF}12.34} &
  \multicolumn{1}{c|}{\cellcolor[HTML]{FFFFFF}20.74} &
  88.5 &
  \multicolumn{1}{c|}{\cellcolor[HTML]{FFFFFF}16} &
  \multicolumn{1}{c|}{\cellcolor[HTML]{FFFFFF}499} &
  96 \\ \hline
3 &
  400 &
  \multicolumn{1}{c|}{\cellcolor[HTML]{FFFFFF}242} &
  \multicolumn{1}{c|}{\cellcolor[HTML]{FFFFFF}158} &
  0 &
  \multicolumn{1}{c|}{\cellcolor[HTML]{FFFFFF}59.6} &
  \multicolumn{1}{c|}{\cellcolor[HTML]{FFFFFF}13.8} &
  \multicolumn{1}{c|}{\cellcolor[HTML]{FFFFFF}18} &
  94 &
  \multicolumn{1}{c|}{\cellcolor[HTML]{FFFFFF}62.3} &
  \multicolumn{1}{c|}{\cellcolor[HTML]{FFFFFF}12.9} &
  \multicolumn{1}{c|}{\cellcolor[HTML]{FFFFFF}19} &
  89 &
  \multicolumn{1}{c|}{\cellcolor[HTML]{FFFFFF}24} &
  \multicolumn{1}{c|}{\cellcolor[HTML]{FFFFFF}376} &
  0 \\ \hline
4 &
  221 &
  \multicolumn{1}{c|}{\cellcolor[HTML]{FFFFFF}88} &
  \multicolumn{1}{c|}{\cellcolor[HTML]{FFFFFF}69} &
  64 &
  \multicolumn{1}{c|}{\cellcolor[HTML]{FFFFFF}42.29} &
  \multicolumn{1}{c|}{\cellcolor[HTML]{FFFFFF}16.56} &
  \multicolumn{1}{c|}{\cellcolor[HTML]{FFFFFF}NA} &
  NA &
  \multicolumn{1}{c|}{\cellcolor[HTML]{FFFFFF}37.34} &
  \multicolumn{1}{c|}{\cellcolor[HTML]{FFFFFF}16.43} &
  \multicolumn{1}{c|}{\cellcolor[HTML]{FFFFFF}NA} &
  NA &
  \multicolumn{1}{c|}{\cellcolor[HTML]{FFFFFF}57} &
  \multicolumn{1}{c|}{\cellcolor[HTML]{FFFFFF}72} &
  92 \\ \hline
5 &
  193 &
  \multicolumn{1}{c|}{\cellcolor[HTML]{FFFFFF}92} &
  \multicolumn{1}{c|}{\cellcolor[HTML]{FFFFFF}101} &
  0 &
  \multicolumn{1}{c|}{\cellcolor[HTML]{FFFFFF}56.08} &
  \multicolumn{1}{c|}{\cellcolor[HTML]{FFFFFF}13.42} &
  \multicolumn{1}{c|}{\cellcolor[HTML]{FFFFFF}24} &
  80 &
  \multicolumn{1}{c|}{\cellcolor[HTML]{FFFFFF}52.04} &
  \multicolumn{1}{c|}{\cellcolor[HTML]{FFFFFF}14.99} &
  \multicolumn{1}{c|}{\cellcolor[HTML]{FFFFFF}18} &
  78 &
  \multicolumn{1}{c|}{\cellcolor[HTML]{FFFFFF}45} &
  \multicolumn{1}{c|}{\cellcolor[HTML]{FFFFFF}47} &
  101 \\ \hline
6 &
  120 &
  \multicolumn{1}{c|}{\cellcolor[HTML]{FFFFFF}73} &
  \multicolumn{1}{c|}{\cellcolor[HTML]{FFFFFF}47} &
  0 &
  \multicolumn{1}{c|}{\cellcolor[HTML]{FFFFFF}52.7} &
  \multicolumn{1}{c|}{\cellcolor[HTML]{FFFFFF}15.6} &
  \multicolumn{1}{c|}{\cellcolor[HTML]{FFFFFF}22} &
  81 &
  \multicolumn{1}{c|}{\cellcolor[HTML]{FFFFFF}50.2} &
  \multicolumn{1}{c|}{\cellcolor[HTML]{FFFFFF}15.3} &
  \multicolumn{1}{c|}{\cellcolor[HTML]{FFFFFF}22} &
  71 &
  \multicolumn{1}{c|}{\cellcolor[HTML]{FFFFFF}29} &
  \multicolumn{1}{c|}{\cellcolor[HTML]{FFFFFF}88} &
  3 \\ \hline
7 &
  120 &
  \multicolumn{1}{c|}{\cellcolor[HTML]{FFFFFF}73} &
  \multicolumn{1}{c|}{\cellcolor[HTML]{FFFFFF}47} &
  0 &
  \multicolumn{1}{c|}{\cellcolor[HTML]{FFFFFF}57.1} &
  \multicolumn{1}{c|}{\cellcolor[HTML]{FFFFFF}14.92} &
  \multicolumn{1}{c|}{\cellcolor[HTML]{FFFFFF}24} &
  81 &
  \multicolumn{1}{c|}{\cellcolor[HTML]{FFFFFF}56.42} &
  \multicolumn{1}{c|}{\cellcolor[HTML]{FFFFFF}14.78} &
  \multicolumn{1}{c|}{\cellcolor[HTML]{FFFFFF}21} &
  85 &
  \multicolumn{1}{c|}{\cellcolor[HTML]{FFFFFF}22} &
  \multicolumn{1}{c|}{\cellcolor[HTML]{FFFFFF}98} &
  0 \\ \hline
8 &
  120 &
  \multicolumn{1}{c|}{\cellcolor[HTML]{FFFFFF}72} &
  \multicolumn{1}{c|}{\cellcolor[HTML]{FFFFFF}48} &
  0 &
  \multicolumn{1}{c|}{\cellcolor[HTML]{FFFFFF}59.9} &
  \multicolumn{1}{c|}{\cellcolor[HTML]{FFFFFF}10.25} &
  \multicolumn{1}{c|}{\cellcolor[HTML]{FFFFFF}36} &
  79 &
  \multicolumn{1}{c|}{\cellcolor[HTML]{FFFFFF}61.2} &
  \multicolumn{1}{c|}{\cellcolor[HTML]{FFFFFF}9.59} &
  \multicolumn{1}{c|}{\cellcolor[HTML]{FFFFFF}28} &
  74 &
  \multicolumn{1}{c|}{\cellcolor[HTML]{FFFFFF}3} &
  \multicolumn{1}{c|}{\cellcolor[HTML]{FFFFFF}117} &
  0 \\ \hline
9 &
  118 &
  \multicolumn{1}{c|}{\cellcolor[HTML]{FFFFFF}64} &
  \multicolumn{1}{c|}{\cellcolor[HTML]{FFFFFF}54} &
  0 &
  \multicolumn{1}{c|}{\cellcolor[HTML]{FFFFFF}58.76} &
  \multicolumn{1}{c|}{\cellcolor[HTML]{FFFFFF}11.21} &
  \multicolumn{1}{c|}{\cellcolor[HTML]{FFFFFF}23} &
  77 &
  \multicolumn{1}{c|}{\cellcolor[HTML]{FFFFFF}59.03} &
  \multicolumn{1}{c|}{\cellcolor[HTML]{FFFFFF}10.66} &
  \multicolumn{1}{c|}{\cellcolor[HTML]{FFFFFF}31} &
  77 &
  \multicolumn{1}{c|}{\cellcolor[HTML]{FFFFFF}4} &
  \multicolumn{1}{c|}{\cellcolor[HTML]{FFFFFF}78} &
  36 \\ \hline
10 &
  114 &
  \multicolumn{1}{c|}{\cellcolor[HTML]{FFFFFF}64} &
  \multicolumn{1}{c|}{\cellcolor[HTML]{FFFFFF}50} &
  0 &
  \multicolumn{1}{c|}{\cellcolor[HTML]{FFFFFF}60.95} &
  \multicolumn{1}{c|}{\cellcolor[HTML]{FFFFFF}11.54} &
  \multicolumn{1}{c|}{\cellcolor[HTML]{FFFFFF}30} &
  86 &
  \multicolumn{1}{c|}{\cellcolor[HTML]{FFFFFF}61.14} &
  \multicolumn{1}{c|}{\cellcolor[HTML]{FFFFFF}15} &
  \multicolumn{1}{c|}{\cellcolor[HTML]{FFFFFF}18} &
  85 &
  \multicolumn{1}{c|}{\cellcolor[HTML]{FFFFFF}2} &
  \multicolumn{1}{c|}{\cellcolor[HTML]{FFFFFF}112} &
  0 \\ \hline
11 &
  112 &
  \multicolumn{1}{c|}{\cellcolor[HTML]{FFFFFF}0} &
  \multicolumn{1}{c|}{\cellcolor[HTML]{FFFFFF}0} &
  112 &
  \multicolumn{1}{c|}{\cellcolor[HTML]{FFFFFF}NA} &
  \multicolumn{1}{c|}{\cellcolor[HTML]{FFFFFF}NA} &
  \multicolumn{1}{c|}{\cellcolor[HTML]{FFFFFF}NA} &
  NA &
  \multicolumn{1}{c|}{\cellcolor[HTML]{FFFFFF}NA} &
  \multicolumn{1}{c|}{\cellcolor[HTML]{FFFFFF}NA} &
  \multicolumn{1}{c|}{\cellcolor[HTML]{FFFFFF}NA} &
  NA &
  \multicolumn{1}{c|}{\cellcolor[HTML]{FFFFFF}0} &
  \multicolumn{1}{c|}{\cellcolor[HTML]{FFFFFF}0} &
  112 \\ \hline
12 &
  108 &
  \multicolumn{1}{c|}{\cellcolor[HTML]{FFFFFF}69} &
  \multicolumn{1}{c|}{\cellcolor[HTML]{FFFFFF}39} &
  0 &
  \multicolumn{1}{c|}{\cellcolor[HTML]{FFFFFF}61.15} &
  \multicolumn{1}{c|}{\cellcolor[HTML]{FFFFFF}NA} &
  \multicolumn{1}{c|}{\cellcolor[HTML]{FFFFFF}18} &
  88 &
  \multicolumn{1}{c|}{\cellcolor[HTML]{FFFFFF}60.15} &
  \multicolumn{1}{c|}{\cellcolor[HTML]{FFFFFF}NA} &
  \multicolumn{1}{c|}{\cellcolor[HTML]{FFFFFF}18} &
  88 &
  \multicolumn{1}{c|}{\cellcolor[HTML]{FFFFFF}0} &
  \multicolumn{1}{c|}{\cellcolor[HTML]{FFFFFF}0} &
  108 \\ \hline
13 &
  108 &
  \multicolumn{1}{c|}{\cellcolor[HTML]{FFFFFF}78} &
  \multicolumn{1}{c|}{\cellcolor[HTML]{FFFFFF}30} &
  0 &
  \multicolumn{1}{c|}{\cellcolor[HTML]{FFFFFF}54.3} &
  \multicolumn{1}{c|}{\cellcolor[HTML]{FFFFFF}14.2} &
  \multicolumn{1}{c|}{\cellcolor[HTML]{FFFFFF}24} &
  82 &
  \multicolumn{1}{c|}{\cellcolor[HTML]{FFFFFF}66} &
  \multicolumn{1}{c|}{\cellcolor[HTML]{FFFFFF}9.9} &
  \multicolumn{1}{c|}{\cellcolor[HTML]{FFFFFF}29} &
  85 &
  \multicolumn{1}{c|}{\cellcolor[HTML]{FFFFFF}5} &
  \multicolumn{1}{c|}{\cellcolor[HTML]{FFFFFF}51} &
  52 \\ \hline
14 &
  107 &
  \multicolumn{1}{c|}{\cellcolor[HTML]{FFFFFF}63} &
  \multicolumn{1}{c|}{\cellcolor[HTML]{FFFFFF}44} &
  0 &
  \multicolumn{1}{c|}{\cellcolor[HTML]{FFFFFF}58.36} &
  \multicolumn{1}{c|}{\cellcolor[HTML]{FFFFFF}10.79} &
  \multicolumn{1}{c|}{\cellcolor[HTML]{FFFFFF}29.3} &
  79.1 &
  \multicolumn{1}{c|}{\cellcolor[HTML]{FFFFFF}59.89} &
  \multicolumn{1}{c|}{\cellcolor[HTML]{FFFFFF}10.79} &
  \multicolumn{1}{c|}{\cellcolor[HTML]{FFFFFF}43.1} &
  78.3 &
  \multicolumn{1}{c|}{\cellcolor[HTML]{FFFFFF}2} &
  \multicolumn{1}{c|}{\cellcolor[HTML]{FFFFFF}46} &
  59 \\ \hline
15 &
  104 &
  \multicolumn{1}{c|}{\cellcolor[HTML]{FFFFFF}66} &
  \multicolumn{1}{c|}{\cellcolor[HTML]{FFFFFF}38} &
  0 &
  \multicolumn{1}{c|}{\cellcolor[HTML]{FFFFFF}57.29} &
  \multicolumn{1}{c|}{\cellcolor[HTML]{FFFFFF}15.85} &
  \multicolumn{1}{c|}{\cellcolor[HTML]{FFFFFF}7} &
  86 &
  \multicolumn{1}{c|}{\cellcolor[HTML]{FFFFFF}61.45} &
  \multicolumn{1}{c|}{\cellcolor[HTML]{FFFFFF}16.13} &
  \multicolumn{1}{c|}{\cellcolor[HTML]{FFFFFF}30} &
  87 &
  \multicolumn{1}{c|}{\cellcolor[HTML]{FFFFFF}10} &
  \multicolumn{1}{c|}{\cellcolor[HTML]{FFFFFF}42} &
  52 \\ \hline
16 &
  101 &
  \multicolumn{1}{c|}{\cellcolor[HTML]{FFFFFF}60} &
  \multicolumn{1}{c|}{\cellcolor[HTML]{FFFFFF}41} &
  0 &
  \multicolumn{1}{c|}{\cellcolor[HTML]{FFFFFF}54.89} &
  \multicolumn{1}{c|}{\cellcolor[HTML]{FFFFFF}13.6} &
  \multicolumn{1}{c|}{\cellcolor[HTML]{FFFFFF}27} &
  79 &
  \multicolumn{1}{c|}{\cellcolor[HTML]{FFFFFF}56.9} &
  \multicolumn{1}{c|}{\cellcolor[HTML]{FFFFFF}14.05} &
  \multicolumn{1}{c|}{\cellcolor[HTML]{FFFFFF}25} &
  90 &
  \multicolumn{1}{c|}{\cellcolor[HTML]{FFFFFF}6} &
  \multicolumn{1}{c|}{\cellcolor[HTML]{FFFFFF}35} &
  60 \\ \hline
17 &
  100 &
  \multicolumn{1}{c|}{\cellcolor[HTML]{FFFFFF}65} &
  \multicolumn{1}{c|}{\cellcolor[HTML]{FFFFFF}35} &
  0 &
  \multicolumn{1}{c|}{\cellcolor[HTML]{FFFFFF}61.88} &
  \multicolumn{1}{c|}{\cellcolor[HTML]{FFFFFF}NA} &
  \multicolumn{1}{c|}{\cellcolor[HTML]{FFFFFF}NA} &
  \cellcolor[HTML]{FFFFFF}NA &
  \multicolumn{1}{c|}{\cellcolor[HTML]{FFFFFF}63.44} &
  \multicolumn{1}{c|}{\cellcolor[HTML]{FFFFFF}NA} &
  \multicolumn{1}{c|}{\cellcolor[HTML]{FFFFFF}NA} &
  N/A &
  \multicolumn{1}{c|}{\cellcolor[HTML]{FFFFFF}0} &
  \multicolumn{1}{c|}{\cellcolor[HTML]{FFFFFF}0} &
  100 \\ \hline
18 &
  100 &
  \multicolumn{1}{c|}{\cellcolor[HTML]{FFFFFF}54} &
  \multicolumn{1}{c|}{\cellcolor[HTML]{FFFFFF}46} &
  0 &
  \multicolumn{1}{c|}{\cellcolor[HTML]{FFFFFF}58.22} &
  \multicolumn{1}{c|}{\cellcolor[HTML]{FFFFFF}12.25} &
  \multicolumn{1}{c|}{\cellcolor[HTML]{FFFFFF}27} &
  77 &
  \multicolumn{1}{c|}{\cellcolor[HTML]{FFFFFF}55.93} &
  \multicolumn{1}{c|}{\cellcolor[HTML]{FFFFFF}16.83} &
  \multicolumn{1}{c|}{\cellcolor[HTML]{FFFFFF}19} &
  78 &
  \multicolumn{1}{c|}{\cellcolor[HTML]{FFFFFF}12} &
  \multicolumn{1}{c|}{\cellcolor[HTML]{FFFFFF}88} &
  0 \\ \hline
19 &
  100 &
  \multicolumn{1}{c|}{\cellcolor[HTML]{FFFFFF}69} &
  \multicolumn{1}{c|}{\cellcolor[HTML]{FFFFFF}30} &
  1 &
  \multicolumn{1}{c|}{\cellcolor[HTML]{FFFFFF}60} &
  \multicolumn{1}{c|}{\cellcolor[HTML]{FFFFFF}12.5} &
  \multicolumn{1}{c|}{\cellcolor[HTML]{FFFFFF}25} &
  81 &
  \multicolumn{1}{c|}{\cellcolor[HTML]{FFFFFF}61.7} &
  \multicolumn{1}{c|}{\cellcolor[HTML]{FFFFFF}12.8} &
  \multicolumn{1}{c|}{\cellcolor[HTML]{FFFFFF}36} &
  87 &
  \multicolumn{1}{c|}{\cellcolor[HTML]{FFFFFF}11} &
  \multicolumn{1}{c|}{\cellcolor[HTML]{FFFFFF}88} &
  1 \\ \hline
20 &
  100 &
  \multicolumn{1}{c|}{\cellcolor[HTML]{FFFFFF}62} &
  \multicolumn{1}{c|}{\cellcolor[HTML]{FFFFFF}38} &
  0 &
  \multicolumn{1}{c|}{\cellcolor[HTML]{FFFFFF}64.31} &
  \multicolumn{1}{c|}{\cellcolor[HTML]{FFFFFF}11.82} &
  \multicolumn{1}{c|}{\cellcolor[HTML]{FFFFFF}31} &
  87 &
  \multicolumn{1}{c|}{\cellcolor[HTML]{FFFFFF}61.08} &
  \multicolumn{1}{c|}{\cellcolor[HTML]{FFFFFF}14.41} &
  \multicolumn{1}{c|}{\cellcolor[HTML]{FFFFFF}22} &
  84 &
  \multicolumn{1}{c|}{\cellcolor[HTML]{FFFFFF}9} &
  \multicolumn{1}{c|}{\cellcolor[HTML]{FFFFFF}83} &
  8 \\ \hline
21 &
  100 &
  \multicolumn{1}{c|}{\cellcolor[HTML]{FFFFFF}72} &
  \multicolumn{1}{c|}{\cellcolor[HTML]{FFFFFF}28} &
  0 &
  \multicolumn{1}{c|}{\cellcolor[HTML]{FFFFFF}53.4} &
  \multicolumn{1}{c|}{\cellcolor[HTML]{FFFFFF}15.7} &
  \multicolumn{1}{c|}{\cellcolor[HTML]{FFFFFF}18} &
  84 &
  \multicolumn{1}{c|}{\cellcolor[HTML]{FFFFFF}52.8} &
  \multicolumn{1}{c|}{\cellcolor[HTML]{FFFFFF}15.9} &
  \multicolumn{1}{c|}{\cellcolor[HTML]{FFFFFF}20} &
  84 &
  \multicolumn{1}{c|}{\cellcolor[HTML]{FFFFFF}22} &
  \multicolumn{1}{c|}{\cellcolor[HTML]{FFFFFF}78} &
  0 \\ \hline
22 &
  94 &
  \multicolumn{1}{c|}{\cellcolor[HTML]{FFFFFF}33} &
  \multicolumn{1}{c|}{\cellcolor[HTML]{FFFFFF}34} &
  27 &
  \multicolumn{1}{c|}{\cellcolor[HTML]{FFFFFF}56.3} &
  \multicolumn{1}{c|}{\cellcolor[HTML]{FFFFFF}12.4} &
  \multicolumn{1}{c|}{\cellcolor[HTML]{FFFFFF}29.17} &
  79.31 &
  \multicolumn{1}{c|}{\cellcolor[HTML]{FFFFFF}60.13} &
  \multicolumn{1}{c|}{\cellcolor[HTML]{FFFFFF}15.09} &
  \multicolumn{1}{c|}{\cellcolor[HTML]{FFFFFF}23.27} &
  83.66 &
  \multicolumn{1}{c|}{\cellcolor[HTML]{FFFFFF}7} &
  \multicolumn{1}{c|}{\cellcolor[HTML]{FFFFFF}56} &
  31 \\ \hline
23 &
  93 &
  \multicolumn{1}{c|}{\cellcolor[HTML]{FFFFFF}51} &
  \multicolumn{1}{c|}{\cellcolor[HTML]{FFFFFF}42} &
  0 &
  \multicolumn{1}{c|}{\cellcolor[HTML]{FFFFFF}51.05} &
  \multicolumn{1}{c|}{\cellcolor[HTML]{FFFFFF}NA} &
  \multicolumn{1}{c|}{\cellcolor[HTML]{FFFFFF}NA} &
  NA &
  \multicolumn{1}{c|}{\cellcolor[HTML]{FFFFFF}57} &
  \multicolumn{1}{c|}{\cellcolor[HTML]{FFFFFF}NA} &
  \multicolumn{1}{c|}{\cellcolor[HTML]{FFFFFF}NA} &
  NA &
  \multicolumn{1}{c|}{\cellcolor[HTML]{FFFFFF}15} &
  \multicolumn{1}{c|}{\cellcolor[HTML]{FFFFFF}78} &
  0 \\ \hline
24 &
  90 &
  \multicolumn{1}{c|}{\cellcolor[HTML]{FFFFFF}47} &
  \multicolumn{1}{c|}{\cellcolor[HTML]{FFFFFF}43} &
  0 &
  \multicolumn{1}{c|}{\cellcolor[HTML]{FFFFFF}55} &
  \multicolumn{1}{c|}{\cellcolor[HTML]{FFFFFF}16} &
  \multicolumn{1}{c|}{\cellcolor[HTML]{FFFFFF}13} &
  86 &
  \multicolumn{1}{c|}{\cellcolor[HTML]{FFFFFF}62} &
  \multicolumn{1}{c|}{\cellcolor[HTML]{FFFFFF}11} &
  \multicolumn{1}{c|}{\cellcolor[HTML]{FFFFFF}28} &
  81 &
  \multicolumn{1}{c|}{\cellcolor[HTML]{FFFFFF}5} &
  \multicolumn{1}{c|}{\cellcolor[HTML]{FFFFFF}85} &
  0 \\ \hline
25 &
  89 &
  \multicolumn{1}{c|}{\cellcolor[HTML]{FFFFFF}47} &
  \multicolumn{1}{c|}{\cellcolor[HTML]{FFFFFF}42} &
  0 &
  \multicolumn{1}{c|}{\cellcolor[HTML]{FFFFFF}61.45} &
  \multicolumn{1}{c|}{\cellcolor[HTML]{FFFFFF}11.73} &
  \multicolumn{1}{c|}{\cellcolor[HTML]{FFFFFF}34} &
  80 &
  \multicolumn{1}{c|}{\cellcolor[HTML]{FFFFFF}65.97} &
  \multicolumn{1}{c|}{\cellcolor[HTML]{FFFFFF}10.56} &
  \multicolumn{1}{c|}{\cellcolor[HTML]{FFFFFF}23} &
  79 &
  \multicolumn{1}{c|}{\cellcolor[HTML]{FFFFFF}9} &
  \multicolumn{1}{c|}{\cellcolor[HTML]{FFFFFF}27} &
  53 \\ \hline
26 &
  85 &
  \multicolumn{1}{c|}{\cellcolor[HTML]{FFFFFF}0} &
  \multicolumn{1}{c|}{\cellcolor[HTML]{FFFFFF}0} &
  85 &
  \multicolumn{1}{c|}{\cellcolor[HTML]{FFFFFF}NA} &
  \multicolumn{1}{c|}{\cellcolor[HTML]{FFFFFF}NA} &
  \multicolumn{1}{c|}{\cellcolor[HTML]{FFFFFF}NA} &
  NA &
  \multicolumn{1}{c|}{\cellcolor[HTML]{FFFFFF}NA} &
  \multicolumn{1}{c|}{\cellcolor[HTML]{FFFFFF}NA} &
  \multicolumn{1}{c|}{\cellcolor[HTML]{FFFFFF}NA} &
  NA &
  \multicolumn{1}{c|}{\cellcolor[HTML]{FFFFFF}0} &
  \multicolumn{1}{c|}{\cellcolor[HTML]{FFFFFF}0} &
  85 \\ \hline
27 &
  85 &
  \multicolumn{1}{c|}{\cellcolor[HTML]{FFFFFF}58} &
  \multicolumn{1}{c|}{\cellcolor[HTML]{FFFFFF}27} &
  0 &
  \multicolumn{1}{c|}{\cellcolor[HTML]{FFFFFF}63.36} &
  \multicolumn{1}{c|}{\cellcolor[HTML]{FFFFFF}10.49} &
  \multicolumn{1}{c|}{\cellcolor[HTML]{FFFFFF}34} &
  83 &
  \multicolumn{1}{c|}{\cellcolor[HTML]{FFFFFF}59.81} &
  \multicolumn{1}{c|}{\cellcolor[HTML]{FFFFFF}10.69} &
  \multicolumn{1}{c|}{\cellcolor[HTML]{FFFFFF}29} &
  82 &
  \multicolumn{1}{c|}{\cellcolor[HTML]{FFFFFF}5} &
  \multicolumn{1}{c|}{\cellcolor[HTML]{FFFFFF}53} &
  27 \\ \hline
28 &
  84 &
  \multicolumn{1}{c|}{\cellcolor[HTML]{FFFFFF}42} &
  \multicolumn{1}{c|}{\cellcolor[HTML]{FFFFFF}42} &
  0 &
  \multicolumn{1}{c|}{\cellcolor[HTML]{FFFFFF}61.03} &
  \multicolumn{1}{c|}{\cellcolor[HTML]{FFFFFF}13.64} &
  \multicolumn{1}{c|}{\cellcolor[HTML]{FFFFFF}12.08} &
  87.78 &
  \multicolumn{1}{c|}{\cellcolor[HTML]{FFFFFF}63.35} &
  \multicolumn{1}{c|}{\cellcolor[HTML]{FFFFFF}13.51} &
  \multicolumn{1}{c|}{\cellcolor[HTML]{FFFFFF}12.13} &
  82.08 &
  \multicolumn{1}{c|}{\cellcolor[HTML]{FFFFFF}3} &
  \multicolumn{1}{c|}{\cellcolor[HTML]{FFFFFF}81} &
  0 \\ \hline
29 &
  81 &
  \multicolumn{1}{c|}{\cellcolor[HTML]{FFFFFF}52} &
  \multicolumn{1}{c|}{\cellcolor[HTML]{FFFFFF}29} &
  0 &
  \multicolumn{1}{c|}{\cellcolor[HTML]{FFFFFF}59.3} &
  \multicolumn{1}{c|}{\cellcolor[HTML]{FFFFFF}NA} &
  \multicolumn{1}{c|}{\cellcolor[HTML]{FFFFFF}NA} &
  NA &
  \multicolumn{1}{c|}{\cellcolor[HTML]{FFFFFF}58.2} &
  \multicolumn{1}{c|}{\cellcolor[HTML]{FFFFFF}NA} &
  \multicolumn{1}{c|}{\cellcolor[HTML]{FFFFFF}NA} &
  NA &
  \multicolumn{1}{c|}{\cellcolor[HTML]{FFFFFF}3} &
  \multicolumn{1}{c|}{\cellcolor[HTML]{FFFFFF}51} &
  27 \\ \hline
30 &
  81 &
  \multicolumn{1}{c|}{\cellcolor[HTML]{FFFFFF}47} &
  \multicolumn{1}{c|}{\cellcolor[HTML]{FFFFFF}34} &
  0 &
  \multicolumn{1}{c|}{\cellcolor[HTML]{FFFFFF}62} &
  \multicolumn{1}{c|}{\cellcolor[HTML]{FFFFFF}12} &
  \multicolumn{1}{c|}{\cellcolor[HTML]{FFFFFF}16} &
  84 &
  \multicolumn{1}{c|}{\cellcolor[HTML]{FFFFFF}59} &
  \multicolumn{1}{c|}{\cellcolor[HTML]{FFFFFF}11} &
  \multicolumn{1}{c|}{\cellcolor[HTML]{FFFFFF}33} &
  80 &
  \multicolumn{1}{c|}{\cellcolor[HTML]{FFFFFF}0} &
  \multicolumn{1}{c|}{\cellcolor[HTML]{FFFFFF}0} &
  81 \\ \hline
31 &
  80 &
  \multicolumn{1}{c|}{\cellcolor[HTML]{FFFFFF}49} &
  \multicolumn{1}{c|}{\cellcolor[HTML]{FFFFFF}31} &
  0 &
  \multicolumn{1}{c|}{\cellcolor[HTML]{FFFFFF}51.66} &
  \multicolumn{1}{c|}{\cellcolor[HTML]{FFFFFF}14.39} &
  \multicolumn{1}{c|}{\cellcolor[HTML]{FFFFFF}15} &
  81 &
  \multicolumn{1}{c|}{\cellcolor[HTML]{FFFFFF}50} &
  \multicolumn{1}{c|}{\cellcolor[HTML]{FFFFFF}12.33} &
  \multicolumn{1}{c|}{\cellcolor[HTML]{FFFFFF}21} &
  69 &
  \multicolumn{1}{c|}{\cellcolor[HTML]{FFFFFF}1} &
  \multicolumn{1}{c|}{\cellcolor[HTML]{FFFFFF}14} &
  65 \\ \hline
32 &
  80 &
  \multicolumn{1}{c|}{\cellcolor[HTML]{FFFFFF}57} &
  \multicolumn{1}{c|}{\cellcolor[HTML]{FFFFFF}23} &
  0 &
  \multicolumn{1}{c|}{\cellcolor[HTML]{FFFFFF}55.53} &
  \multicolumn{1}{c|}{\cellcolor[HTML]{FFFFFF}11.96} &
  \multicolumn{1}{c|}{\cellcolor[HTML]{FFFFFF}34} &
  81 &
  \multicolumn{1}{c|}{\cellcolor[HTML]{FFFFFF}53.57} &
  \multicolumn{1}{c|}{\cellcolor[HTML]{FFFFFF}11.96} &
  \multicolumn{1}{c|}{\cellcolor[HTML]{FFFFFF}32} &
  79 &
  \multicolumn{1}{c|}{\cellcolor[HTML]{FFFFFF}5} &
  \multicolumn{1}{c|}{\cellcolor[HTML]{FFFFFF}66} &
  9 \\ \hline
33 &
  78 &
  \multicolumn{1}{c|}{\cellcolor[HTML]{FFFFFF}47} &
  \multicolumn{1}{c|}{\cellcolor[HTML]{FFFFFF}31} &
  0 &
  \multicolumn{1}{c|}{\cellcolor[HTML]{FFFFFF}58.9} &
  \multicolumn{1}{c|}{\cellcolor[HTML]{FFFFFF}10.69} &
  \multicolumn{1}{c|}{\cellcolor[HTML]{FFFFFF}22.52} &
  76.58 &
  \multicolumn{1}{c|}{\cellcolor[HTML]{FFFFFF}59.4} &
  \multicolumn{1}{c|}{\cellcolor[HTML]{FFFFFF}11.06} &
  \multicolumn{1}{c|}{\cellcolor[HTML]{FFFFFF}30.25} &
  81.7 &
  \multicolumn{1}{c|}{\cellcolor[HTML]{FFFFFF}4} &
  \multicolumn{1}{c|}{\cellcolor[HTML]{FFFFFF}71} &
  3 \\ \hline
34 &
  70 &
  \multicolumn{1}{c|}{\cellcolor[HTML]{FFFFFF}45} &
  \multicolumn{1}{c|}{\cellcolor[HTML]{FFFFFF}25} &
  0 &
  \multicolumn{1}{c|}{\cellcolor[HTML]{FFFFFF}NA} &
  \multicolumn{1}{c|}{\cellcolor[HTML]{FFFFFF}NA} &
  \multicolumn{1}{c|}{\cellcolor[HTML]{FFFFFF}NA} &
  NA &
  \multicolumn{1}{c|}{\cellcolor[HTML]{FFFFFF}NA} &
  \multicolumn{1}{c|}{\cellcolor[HTML]{FFFFFF}NA} &
  \multicolumn{1}{c|}{\cellcolor[HTML]{FFFFFF}NA} &
  NA &
  \multicolumn{1}{c|}{\cellcolor[HTML]{FFFFFF}0} &
  \multicolumn{1}{c|}{\cellcolor[HTML]{FFFFFF}0} &
  70 \\ \hline
35 &
  70 &
  \multicolumn{1}{c|}{\cellcolor[HTML]{FFFFFF}45} &
  \multicolumn{1}{c|}{\cellcolor[HTML]{FFFFFF}25} &
  0 &
  \multicolumn{1}{c|}{\cellcolor[HTML]{FFFFFF}64.17} &
  \multicolumn{1}{c|}{\cellcolor[HTML]{FFFFFF}9.79} &
  \multicolumn{1}{c|}{\cellcolor[HTML]{FFFFFF}40} &
  85 &
  \multicolumn{1}{c|}{\cellcolor[HTML]{FFFFFF}63.8} &
  \multicolumn{1}{c|}{\cellcolor[HTML]{FFFFFF}11.35} &
  \multicolumn{1}{c|}{\cellcolor[HTML]{FFFFFF}35} &
  83 &
  \multicolumn{1}{c|}{\cellcolor[HTML]{FFFFFF}6} &
  \multicolumn{1}{c|}{\cellcolor[HTML]{FFFFFF}61} &
  3 \\ \hline
36 &
  67 &
  \multicolumn{1}{c|}{\cellcolor[HTML]{FFFFFF}39} &
  \multicolumn{1}{c|}{\cellcolor[HTML]{FFFFFF}28} &
  0 &
  \multicolumn{1}{c|}{\cellcolor[HTML]{FFFFFF}64.1} &
  \multicolumn{1}{c|}{\cellcolor[HTML]{FFFFFF}11.6} &
  \multicolumn{1}{c|}{\cellcolor[HTML]{FFFFFF}44} &
  87 &
  \multicolumn{1}{c|}{\cellcolor[HTML]{FFFFFF}60.5} &
  \multicolumn{1}{c|}{\cellcolor[HTML]{FFFFFF}13.1} &
  \multicolumn{1}{c|}{\cellcolor[HTML]{FFFFFF}28} &
  83 &
  \multicolumn{1}{c|}{\cellcolor[HTML]{FFFFFF}5} &
  \multicolumn{1}{c|}{\cellcolor[HTML]{FFFFFF}50} &
  12 \\ \hline
37 &
  66 &
  \multicolumn{1}{c|}{\cellcolor[HTML]{FFFFFF}48} &
  \multicolumn{1}{c|}{\cellcolor[HTML]{FFFFFF}18} &
  0 &
  \multicolumn{1}{c|}{\cellcolor[HTML]{FFFFFF}65.0} &
  \multicolumn{1}{c|}{\cellcolor[HTML]{FFFFFF}14.7} &
  \multicolumn{1}{c|}{\cellcolor[HTML]{FFFFFF}36} &
  91 &
  \multicolumn{1}{c|}{\cellcolor[HTML]{FFFFFF}60.6} &
  \multicolumn{1}{c|}{\cellcolor[HTML]{FFFFFF}10.3} &
  \multicolumn{1}{c|}{\cellcolor[HTML]{FFFFFF}36} &
  70 &
  \multicolumn{1}{c|}{\cellcolor[HTML]{FFFFFF}0} &
  \multicolumn{1}{c|}{\cellcolor[HTML]{FFFFFF}0} &
  66 \\ \hline
38 &
  65 &
  \multicolumn{1}{c|}{\cellcolor[HTML]{FFFFFF}30} &
  \multicolumn{1}{c|}{\cellcolor[HTML]{FFFFFF}35} &
  0 &
  \multicolumn{1}{c|}{\cellcolor[HTML]{FFFFFF}61.23} &
  \multicolumn{1}{c|}{\cellcolor[HTML]{FFFFFF}14.47} &
  \multicolumn{1}{c|}{\cellcolor[HTML]{FFFFFF}30} &
  85 &
  \multicolumn{1}{c|}{\cellcolor[HTML]{FFFFFF}61.85} &
  \multicolumn{1}{c|}{\cellcolor[HTML]{FFFFFF}14.5} &
  \multicolumn{1}{c|}{\cellcolor[HTML]{FFFFFF}29} &
  84 &
  \multicolumn{1}{c|}{\cellcolor[HTML]{FFFFFF}0} &
  \multicolumn{1}{c|}{\cellcolor[HTML]{FFFFFF}50} &
  15 \\ \hline
39 &
  65 &
  \multicolumn{1}{c|}{\cellcolor[HTML]{FFFFFF}38} &
  \multicolumn{1}{c|}{\cellcolor[HTML]{FFFFFF}25} &
  2 &
  \multicolumn{1}{c|}{\cellcolor[HTML]{FFFFFF}57.16} &
  \multicolumn{1}{c|}{\cellcolor[HTML]{FFFFFF}13.51} &
  \multicolumn{1}{c|}{\cellcolor[HTML]{FFFFFF}20} &
  79 &
  \multicolumn{1}{c|}{\cellcolor[HTML]{FFFFFF}60.44} &
  \multicolumn{1}{c|}{\cellcolor[HTML]{FFFFFF}13.01} &
  \multicolumn{1}{c|}{\cellcolor[HTML]{FFFFFF}19} &
  81 &
  \multicolumn{1}{c|}{\cellcolor[HTML]{FFFFFF}2} &
  \multicolumn{1}{c|}{\cellcolor[HTML]{FFFFFF}29} &
  34 \\ \hline
40 &
  64 &
  \multicolumn{1}{c|}{\cellcolor[HTML]{FFFFFF}36} &
  \multicolumn{1}{c|}{\cellcolor[HTML]{FFFFFF}27} &
  1 &
  \multicolumn{1}{c|}{\cellcolor[HTML]{FFFFFF}61.03} &
  \multicolumn{1}{c|}{\cellcolor[HTML]{FFFFFF}11.04} &
  \multicolumn{1}{c|}{\cellcolor[HTML]{FFFFFF}38} &
  81 &
  \multicolumn{1}{c|}{\cellcolor[HTML]{FFFFFF}60.63} &
  \multicolumn{1}{c|}{\cellcolor[HTML]{FFFFFF}11.4} &
  \multicolumn{1}{c|}{\cellcolor[HTML]{FFFFFF}36} &
  82 &
  \multicolumn{1}{c|}{\cellcolor[HTML]{FFFFFF}0} &
  \multicolumn{1}{c|}{\cellcolor[HTML]{FFFFFF}64} &
  0 \\ \hline
41 &
  64 &
  \multicolumn{1}{c|}{\cellcolor[HTML]{FFFFFF}24} &
  \multicolumn{1}{c|}{\cellcolor[HTML]{FFFFFF}16} &
  \cellcolor[HTML]{FFFFFF}24 &
  \multicolumn{1}{c|}{\cellcolor[HTML]{FFFFFF}NA} &
  \multicolumn{1}{c|}{\cellcolor[HTML]{FFFFFF}NA} &
  \multicolumn{1}{c|}{\cellcolor[HTML]{FFFFFF}NA} &
  NA &
  \multicolumn{1}{c|}{\cellcolor[HTML]{FFFFFF}NA} &
  \multicolumn{1}{c|}{\cellcolor[HTML]{FFFFFF}NA} &
  \multicolumn{1}{c|}{\cellcolor[HTML]{FFFFFF}NA} &
  NA &
  \multicolumn{1}{c|}{\cellcolor[HTML]{FFFFFF}0} &
  \multicolumn{1}{c|}{\cellcolor[HTML]{FFFFFF}0} &
  64 \\ \hline
42 &
  59 &
  \multicolumn{1}{c|}{\cellcolor[HTML]{FFFFFF}37} &
  \multicolumn{1}{c|}{\cellcolor[HTML]{FFFFFF}22} &
  0 &
  \multicolumn{1}{c|}{\cellcolor[HTML]{FFFFFF}61.9} &
  \multicolumn{1}{c|}{\cellcolor[HTML]{FFFFFF}12.7} &
  \multicolumn{1}{c|}{\cellcolor[HTML]{FFFFFF}20} &
  91 &
  \multicolumn{1}{c|}{\cellcolor[HTML]{FFFFFF}64.2} &
  \multicolumn{1}{c|}{\cellcolor[HTML]{FFFFFF}10.7} &
  \multicolumn{1}{c|}{\cellcolor[HTML]{FFFFFF}32} &
  74 &
  \multicolumn{1}{c|}{\cellcolor[HTML]{FFFFFF}1} &
  \multicolumn{1}{c|}{\cellcolor[HTML]{FFFFFF}58} &
  0 \\ \hline
43 &
  58 &
  \multicolumn{1}{c|}{\cellcolor[HTML]{FFFFFF}36} &
  \multicolumn{1}{c|}{\cellcolor[HTML]{FFFFFF}19} &
  3 &
  \multicolumn{1}{c|}{\cellcolor[HTML]{FFFFFF}54.36} &
  \multicolumn{1}{c|}{\cellcolor[HTML]{FFFFFF}13.13} &
  \multicolumn{1}{c|}{\cellcolor[HTML]{FFFFFF}20} &
  76 &
  \multicolumn{1}{c|}{\cellcolor[HTML]{FFFFFF}55.79} &
  \multicolumn{1}{c|}{\cellcolor[HTML]{FFFFFF}14.21} &
  \multicolumn{1}{c|}{\cellcolor[HTML]{FFFFFF}24} &
  75 &
  \multicolumn{1}{c|}{\cellcolor[HTML]{FFFFFF}5} &
  \multicolumn{1}{c|}{\cellcolor[HTML]{FFFFFF}53} &
  0 \\ \hline
44 &
  51 &
  \multicolumn{1}{c|}{\cellcolor[HTML]{FFFFFF}33} &
  \multicolumn{1}{c|}{\cellcolor[HTML]{FFFFFF}18} &
  0 &
  \multicolumn{1}{c|}{\cellcolor[HTML]{FFFFFF}55.1} &
  \multicolumn{1}{c|}{\cellcolor[HTML]{FFFFFF}11.8} &
  \multicolumn{1}{c|}{\cellcolor[HTML]{FFFFFF}35} &
  77 &
  \multicolumn{1}{c|}{\cellcolor[HTML]{FFFFFF}61.6} &
  \multicolumn{1}{c|}{\cellcolor[HTML]{FFFFFF}12.3} &
  \multicolumn{1}{c|}{\cellcolor[HTML]{FFFFFF}37} &
  80 &
  \multicolumn{1}{c|}{\cellcolor[HTML]{FFFFFF}1} &
  \multicolumn{1}{c|}{\cellcolor[HTML]{FFFFFF}50} &
  0 \\ \hline
45 &
  50 &
  \multicolumn{1}{c|}{\cellcolor[HTML]{FFFFFF}35} &
  \multicolumn{1}{c|}{\cellcolor[HTML]{FFFFFF}10} &
  5 &
  \multicolumn{1}{c|}{\cellcolor[HTML]{FFFFFF}NA} &
  \multicolumn{1}{c|}{\cellcolor[HTML]{FFFFFF}NA} &
  \multicolumn{1}{c|}{\cellcolor[HTML]{FFFFFF}NA} &
  NA &
  \multicolumn{1}{c|}{\cellcolor[HTML]{FFFFFF}NA} &
  \multicolumn{1}{c|}{\cellcolor[HTML]{FFFFFF}NA} &
  \multicolumn{1}{c|}{\cellcolor[HTML]{FFFFFF}NA} &
  NA &
  \multicolumn{1}{c|}{\cellcolor[HTML]{FFFFFF}0} &
  \multicolumn{1}{c|}{\cellcolor[HTML]{FFFFFF}0} &
  50 \\ \hline
46 &
  48 &
  \multicolumn{1}{c|}{\cellcolor[HTML]{FFFFFF}27} &
  \multicolumn{1}{c|}{\cellcolor[HTML]{FFFFFF}21} &
  0 &
  \multicolumn{1}{c|}{\cellcolor[HTML]{FFFFFF}56.23} &
  \multicolumn{1}{c|}{\cellcolor[HTML]{FFFFFF}12.86} &
  \multicolumn{1}{c|}{\cellcolor[HTML]{FFFFFF}27} &
  80.3 &
  \multicolumn{1}{c|}{\cellcolor[HTML]{FFFFFF}57.84} &
  \multicolumn{1}{c|}{\cellcolor[HTML]{FFFFFF}11.64} &
  \multicolumn{1}{c|}{\cellcolor[HTML]{FFFFFF}35} &
  76.31 &
  \multicolumn{1}{c|}{\cellcolor[HTML]{FFFFFF}0} &
  \multicolumn{1}{c|}{\cellcolor[HTML]{FFFFFF}0} &
  48 \\ \hline
48 &
  46 &
  \multicolumn{1}{c|}{\cellcolor[HTML]{FFFFFF}24} &
  \multicolumn{1}{c|}{\cellcolor[HTML]{FFFFFF}22} &
  0 &
  \multicolumn{1}{c|}{\cellcolor[HTML]{FFFFFF}50.79} &
  \multicolumn{1}{c|}{\cellcolor[HTML]{FFFFFF}14.39} &
  \multicolumn{1}{c|}{\cellcolor[HTML]{FFFFFF}19} &
  72 &
  \multicolumn{1}{c|}{\cellcolor[HTML]{FFFFFF}49.68} &
  \multicolumn{1}{c|}{\cellcolor[HTML]{FFFFFF}18.46} &
  \multicolumn{1}{c|}{\cellcolor[HTML]{FFFFFF}19} &
  79 &
  \multicolumn{1}{c|}{\cellcolor[HTML]{FFFFFF}2} &
  \multicolumn{1}{c|}{\cellcolor[HTML]{FFFFFF}10} &
  34 \\ \hline
49 &
  46 &
  \multicolumn{1}{c|}{\cellcolor[HTML]{FFFFFF}20} &
  \multicolumn{1}{c|}{\cellcolor[HTML]{FFFFFF}12} &
  14 &
  \multicolumn{1}{c|}{\cellcolor[HTML]{FFFFFF}58.25} &
  \multicolumn{1}{c|}{\cellcolor[HTML]{FFFFFF}11.29} &
  \multicolumn{1}{c|}{\cellcolor[HTML]{FFFFFF}28} &
  82 &
  \multicolumn{1}{c|}{\cellcolor[HTML]{FFFFFF}55.67} &
  \multicolumn{1}{c|}{\cellcolor[HTML]{FFFFFF}13.32} &
  \multicolumn{1}{c|}{\cellcolor[HTML]{FFFFFF}25} &
  72 &
  \multicolumn{1}{c|}{\cellcolor[HTML]{FFFFFF}0} &
  \multicolumn{1}{c|}{\cellcolor[HTML]{FFFFFF}3} &
  43 \\ \hline
50 &
  43 &
  \multicolumn{1}{c|}{\cellcolor[HTML]{FFFFFF}24} &
  \multicolumn{1}{c|}{\cellcolor[HTML]{FFFFFF}19} &
  0 &
  \multicolumn{1}{c|}{\cellcolor[HTML]{FFFFFF}NA} &
  \multicolumn{1}{c|}{\cellcolor[HTML]{FFFFFF}NA} &
  \multicolumn{1}{c|}{\cellcolor[HTML]{FFFFFF}31} &
  82 &
  \multicolumn{1}{c|}{\cellcolor[HTML]{FFFFFF}NA} &
  \multicolumn{1}{c|}{\cellcolor[HTML]{FFFFFF}NA} &
  \multicolumn{1}{c|}{\cellcolor[HTML]{FFFFFF}31} &
  82 &
  \multicolumn{1}{c|}{\cellcolor[HTML]{FFFFFF}0} &
  \multicolumn{1}{c|}{\cellcolor[HTML]{FFFFFF}0} &
  43 \\ \hline
52 &
  32 &
  \multicolumn{1}{c|}{\cellcolor[HTML]{FFFFFF}17} &
  \multicolumn{1}{c|}{\cellcolor[HTML]{FFFFFF}15} &
  0 &
  \multicolumn{1}{c|}{\cellcolor[HTML]{FFFFFF}58.8} &
  \multicolumn{1}{c|}{\cellcolor[HTML]{FFFFFF}10.4} &
  \multicolumn{1}{c|}{\cellcolor[HTML]{FFFFFF}35} &
  81 &
  \multicolumn{1}{c|}{\cellcolor[HTML]{FFFFFF}59.6} &
  \multicolumn{1}{c|}{\cellcolor[HTML]{FFFFFF}12.6} &
  \multicolumn{1}{c|}{\cellcolor[HTML]{FFFFFF}31} &
  78 &
  \multicolumn{1}{c|}{\cellcolor[HTML]{FFFFFF}1} &
  \multicolumn{1}{c|}{\cellcolor[HTML]{FFFFFF}4} &
  27 \\ \hline
53 &
  30 &
  \multicolumn{1}{c|}{\cellcolor[HTML]{FFFFFF}0} &
  \multicolumn{1}{c|}{\cellcolor[HTML]{FFFFFF}0} &
  30 &
  \multicolumn{1}{c|}{\cellcolor[HTML]{FFFFFF}NA} &
  \multicolumn{1}{c|}{\cellcolor[HTML]{FFFFFF}NA} &
  \multicolumn{1}{c|}{\cellcolor[HTML]{FFFFFF}NA} &
  NA &
  \multicolumn{1}{c|}{\cellcolor[HTML]{FFFFFF}NA} &
  \multicolumn{1}{c|}{\cellcolor[HTML]{FFFFFF}NA} &
  \multicolumn{1}{c|}{\cellcolor[HTML]{FFFFFF}NA} &
  NA &
  \multicolumn{1}{c|}{\cellcolor[HTML]{FFFFFF}0} &
  \multicolumn{1}{c|}{\cellcolor[HTML]{FFFFFF}0} &
  30 \\ \hline
54 &
  25 &
  \multicolumn{1}{c|}{\cellcolor[HTML]{FFFFFF}0} &
  \multicolumn{1}{c|}{\cellcolor[HTML]{FFFFFF}0} &
  25 &
  \multicolumn{1}{c|}{\cellcolor[HTML]{FFFFFF}58.21} &
  \multicolumn{1}{c|}{\cellcolor[HTML]{FFFFFF}12.42} &
  \multicolumn{1}{c|}{\cellcolor[HTML]{FFFFFF}44.33} &
  75.32 &
  \multicolumn{1}{c|}{\cellcolor[HTML]{FFFFFF}58.21} &
  \multicolumn{1}{c|}{\cellcolor[HTML]{FFFFFF}12.42} &
  \multicolumn{1}{c|}{\cellcolor[HTML]{FFFFFF}44.33} &
  75.32 &
  \multicolumn{1}{c|}{\cellcolor[HTML]{FFFFFF}0} &
  \multicolumn{1}{c|}{\cellcolor[HTML]{FFFFFF}0} &
  25 \\ \hline
56 &
  23 &
  \multicolumn{1}{c|}{\cellcolor[HTML]{FFFFFF}11} &
  \multicolumn{1}{c|}{\cellcolor[HTML]{FFFFFF}12} &
  0 &
  \multicolumn{1}{c|}{\cellcolor[HTML]{FFFFFF}35.09} &
  \multicolumn{1}{c|}{\cellcolor[HTML]{FFFFFF}17.34} &
  \multicolumn{1}{c|}{\cellcolor[HTML]{FFFFFF}7} &
  57 &
  \multicolumn{1}{c|}{\cellcolor[HTML]{FFFFFF}42.16} &
  \multicolumn{1}{c|}{\cellcolor[HTML]{FFFFFF}22.19} &
  \multicolumn{1}{c|}{\cellcolor[HTML]{FFFFFF}5} &
  76 &
  \multicolumn{1}{c|}{\cellcolor[HTML]{FFFFFF}0} &
  \multicolumn{1}{c|}{\cellcolor[HTML]{FFFFFF}0} &
  23 \\ \hline
59 &
  19 &
  \multicolumn{1}{c|}{\cellcolor[HTML]{FFFFFF}0} &
  \multicolumn{1}{c|}{\cellcolor[HTML]{FFFFFF}0} &
  19 &
  \multicolumn{1}{c|}{\cellcolor[HTML]{FFFFFF}NA} &
  \multicolumn{1}{c|}{\cellcolor[HTML]{FFFFFF}NA} &
  \multicolumn{1}{c|}{\cellcolor[HTML]{FFFFFF}NA} &
  NA &
  \multicolumn{1}{c|}{\cellcolor[HTML]{FFFFFF}NA} &
  \multicolumn{1}{c|}{\cellcolor[HTML]{FFFFFF}NA} &
  \multicolumn{1}{c|}{\cellcolor[HTML]{FFFFFF}NA} &
  NA &
  \multicolumn{1}{c|}{\cellcolor[HTML]{FFFFFF}0} &
  \multicolumn{1}{c|}{\cellcolor[HTML]{FFFFFF}0} &
  19 \\ \hline
60 &
  18 &
  \multicolumn{1}{c|}{\cellcolor[HTML]{FFFFFF}12} &
  \multicolumn{1}{c|}{\cellcolor[HTML]{FFFFFF}6} &
  0 &
  \multicolumn{1}{c|}{\cellcolor[HTML]{FFFFFF}50} &
  \multicolumn{1}{c|}{\cellcolor[HTML]{FFFFFF}21} &
  \multicolumn{1}{c|}{\cellcolor[HTML]{FFFFFF}12} &
  72 &
  \multicolumn{1}{c|}{\cellcolor[HTML]{FFFFFF}57} &
  \multicolumn{1}{c|}{\cellcolor[HTML]{FFFFFF}9} &
  \multicolumn{1}{c|}{\cellcolor[HTML]{FFFFFF}43} &
  63 &
  \multicolumn{1}{c|}{\cellcolor[HTML]{FFFFFF}2} &
  \multicolumn{1}{c|}{\cellcolor[HTML]{FFFFFF}9} &
  7 \\ \hline
\begin{tabular}[c]{@{}c@{}}PIM: 47, 51, 55, \\ 57, 58, 61, \\ 62, 63, 64,\\ 65, 66, 67, \\ 68, 69, 70, 71\end{tabular} &
  231 &
  \multicolumn{1}{c|}{\cellcolor[HTML]{FFFFFF}116} &
  \multicolumn{1}{c|}{\cellcolor[HTML]{FFFFFF}92} &
  23 &
  \multicolumn{1}{c|}{\cellcolor[HTML]{FFFFFF}57.02} &
  \multicolumn{1}{c|}{\cellcolor[HTML]{FFFFFF}14.37} &
  \multicolumn{1}{c|}{\cellcolor[HTML]{FFFFFF}17.47} &
  81.21 &
  \multicolumn{1}{c|}{\cellcolor[HTML]{FFFFFF}53.22} &
  \multicolumn{1}{c|}{\cellcolor[HTML]{FFFFFF}14.08} &
  \multicolumn{1}{c|}{\cellcolor[HTML]{FFFFFF}17.7} &
  84.84 &
  \multicolumn{1}{c|}{\cellcolor[HTML]{FFFFFF}0} &
  \multicolumn{1}{c|}{\cellcolor[HTML]{FFFFFF}0} &
  231 \\ \hline
\end{tabular}

\end{adjustbox}

\end{table}
